# Supplementary material for: Large language models in materials science and the need for open-source approaches
Source: arXiv:2511.10673 ancillary file (2025-11-10)
Supplement: Supplementary file 1 [file si.pdf]

# Supporting Information

## Large language models in materials science and the need for open-source approaches

Fengxu Yang<sup>1</sup>, Weitong Chen<sup>2</sup> and Jack D. Evans<sup>\*1</sup>

<sup>1</sup> School of Physics, Chemistry and Earth Sciences, The University of Adelaide

<sup>2</sup> School of Computer and Mathematical Sciences, The University of Adelaide

\*Email: [j.evans@adelaide.edu.au](mailto:j.evans@adelaide.edu.au)

# Contents

|                                           |          |
|-------------------------------------------|----------|
| <b>S1 Synthesis Conditions Extraction</b> | <b>3</b> |
| S1.1 Model Deployment . . . . .           | 3        |
| S1.2 Hardware Requirements . . . . .      | 3        |
| <b>S2 Synthesis Conditions Prediction</b> | <b>4</b> |
| S2.1 Data Analysis . . . . .              | 4        |
| S2.2 Model Fine-tuning . . . . .          | 4        |
| <b>S3 Supplementary References</b>        | <b>6</b> |

# S1 Synthesis Conditions Extraction

## S1.1 Model Deployment

All models evaluated for synthesis condition extraction were deployed locally using the SGLang<sup>1</sup> on Phoenix A100 GPU nodes. Inference was conducted under the officially recommended temperature settings for each model. The complete results are available in the Zenodo repository: [10.5281/zenodo.17548056](https://doi.org/10.5281/zenodo.17548056).

## S1.2 Hardware Requirements

$$\text{VRAM}_{\text{weights}} \approx 2 \text{ GB} \times (\text{billions of parameters})$$

Beyond the model weights themselves, approximately 20% additional VRAM should be allocated for framework overhead and activation storage.

Table S1: VRAM requirements for models tested on synthesis conditions extraction tasks.

| Model                        | Params | VRAM Estimation (GB) |
|------------------------------|--------|----------------------|
| GLM-4.5 (355B)               | 355B   | 852                  |
| Qwen-235B-A30B-Thinking      | 235B   | 564                  |
| GLM-4.5-Air (106GB)          | 106GB  | 254                  |
| Qwen3-Next-80B-A3B-Thinking  | 80B    | 192                  |
| Qwen3-32B                    | 32B    | 77                   |
| DeepSeek-R1-Distill-Qwen-14B | 14B    | 34                   |

**Note:** This estimate excludes the KV cache. When using inference engines like SGLang, additional VRAM will be required to accommodate the KV cache.

## S2 Synthesis Conditions Prediction

### S2.1 Data Analysis

We observed that L2M3’s training dataset is highly unbalanced, as illustrated in Figure S1 by frequency distributions where most parameters are dominated by a single majority class. For example, ‘water’ comprises the vast majority of ‘Solvent’ entries, while ‘False’ dominates ‘pH Adjustment’ cases, resulting in significant data sparsity across all other conditions. Although this imbalance is likely to be representative of real-world experimental distributions, it introduces the challenge for model training to effectively learn from underrepresented examples and achieve robust generalisation.

### S2.2 Model Fine-tuning

The fine-tuning of all models for synthesis condition and test prediction tasks was conducted using the Hugging Face Transformers<sup>2</sup> and PEFT libraries<sup>3</sup>. This process utilised the AMD Instinct MI250X accelerators on the Setonix supercomputer. The models were fine-tuned for 1 epoch using a LoRA rank of 32 to produce the results. A higher rank of 128 was also evaluated and it did not produce significantly different performance. All model inferences were generated using a temperature of 0 using vLLM<sup>4</sup>. The full training script is available in the repository cited earlier.

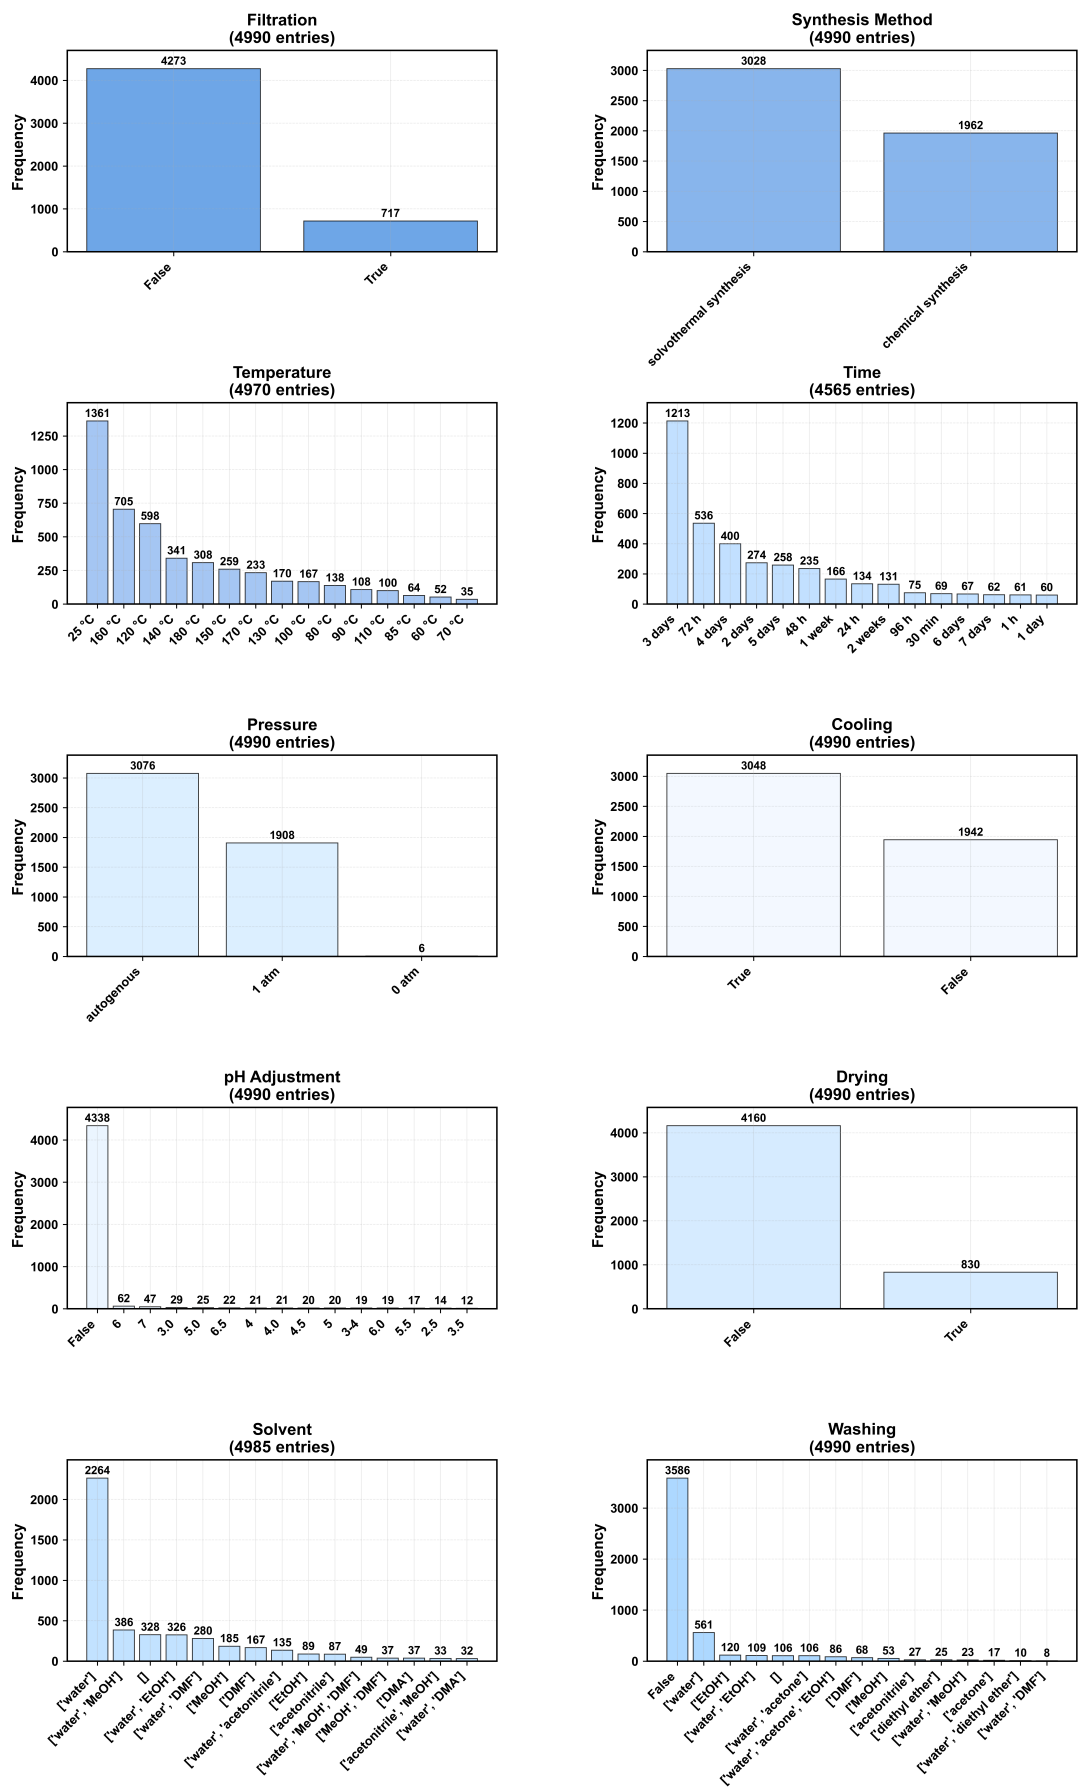

Figure S1: Frequency distribution of the synthesis conditions training dataset from L2M3's code base.

## S3 Supplementary References

### References

- [1] L. Zheng, L. Yin, Z. Xie, C. Sun, J. Huang, C. H. Yu, S. Cao, C. Kozyrakis, I. Stoica, J. E. Gonzalez, C. Barrett and Y. Sheng, *SGLang: Efficient Execution of Structured Language Model Programs*, 2024, <http://arxiv.org/abs/2312.07104>, arXiv:2312.07104.
- [2] T. Wolf, L. Debut, V. Sanh, J. Chaumond, C. Delangue, A. Moi, P. Cistac, T. Rault, R. Louf, M. Funtowicz, J. Davison, S. Shleifer, P. v. Platen, C. Ma, Y. Jernite, J. Plu, C. Xu, T. L. Scao, S. Gugger, M. Drame, Q. Lhoest and A. M. Rush, *HuggingFace’s Transformers: State-of-the-art Natural Language Processing*, 2020, <http://arxiv.org/abs/1910.03771>, arXiv:1910.03771.
- [3] L. Xu, H. Xie, S.-Z. J. Qin, X. Tao and F. L. Wang, *Parameter-Efficient Fine-Tuning Methods for Pretrained Language Models: A Critical Review and Assessment*, 2023, <http://arxiv.org/abs/2312.12148>, arXiv:2312.12148.
- [4] W. Kwon, Z. Li, S. Zhuang, Y. Sheng, L. Zheng, C. H. Yu, J. E. Gonzalez, H. Zhang and I. Stoica, *Proceedings of the ACM SIGOPS 29th Symposium on Operating Systems Principles*, 2023.
